# Supplementary material for: ContactPose: A Dataset of Grasps with Object Contact and Hand Pose
Source: arXiv:2007.09545 source file (2020-07-19)
Supplement: Supplementary file 1 [file data_examples.tex]

\section{Example Data from ContactPose}
\noindent\textbf{RGB-D Images with Projected Hand Pose}: Figure~\ref{fig:data_examples_rgbd} shows example RGB and depth images (256 $\times$ 256 crops centered around the object) for all objects, along with projected 3D joints.

\noindent\textbf{Hand Contact Probabilities}: Figure~\ref{fig:data_examples_hand_contacts} shows (phalange-level) hand-part contact probabilities (similar to Figure 7(b) in the main paper) for all objects, averaged separately over `use' and `hand-off' grasps. Many objects that elicit significantly different `use' and `hand-off' contact patterns, e.g. cellphone, flashlight, hammer, knife, mouse, pan, PS controller, stapler, toothbrush, and toothpaste. The `use' grasps for banana and water-bottle have different contact patterns on the left and right hand, because many participants use their non-dominant hand to hold them firmly in an enveloping grasp and the dominant hand to peel and open the cap, respectively.

\noindent\textbf{Grasps}: To further demonstrate the scale and diversity of ContactPose data, we present a slice of the data. Figures~\ref{fig:data_examples_grasps_use} and~\ref{fig:data_examples_grasps_handoff} show all the `use' and `hand-off' grasps (contact map and hand pose) for one object (PS-controller), respectively. Note the significant influence of intent on grasps, and also the intra-intent diversity of grasps. 

{%
\newcommand{\cameraName}[1]{
    \IfEqCase{#1}{%
        {left}{Kinect\#1}%
        {middle}{Kinect\#2}%
        {right}{Kinect\#3}%
    }[\PackageError{cameraName}{Undefined option to cameraName: #1}{}]%
}

% object, position, mode, angle
\newcommand{\subfigureWithTopCaption}[4]{%
    \captionsetup[subfigure]{labelformat=empty, font=tiny}
    \begin{subfigure}{.15\textwidth}
        \caption{\cameraName{#2}-#3}
        \includegraphics[width=\linewidth, angle=#4, origin=c]{supp_images/rgbd_images/#1_kinect2_#2_#3_use.png}
    \end{subfigure}
}

% object, position, mode, angle
\newcommand{\subfigureWithoutCaption}[4]{%
    \captionsetup[subfigure]{labelformat=empty}
    \begin{subfigure}{.15\textwidth}
        \includegraphics[width=\linewidth, angle=#4, origin=c]{supp_images/rgbd_images/#1_kinect2_#2_#3_use.png}
    \end{subfigure}
}

% object, position, mode, angle
\newcommand{\subfigureWithBottomCaption}[4]{%
    \captionsetup[subfigure]{labelformat=empty, font=tiny}
    \begin{subfigure}{.15\textwidth}
        \includegraphics[width=\linewidth, angle=#4, origin=c]{supp_images/rgbd_images/#1_kinect2_#2_#3_use.png}
        \caption{\cameraName{#2}-#3}
    \end{subfigure}
}

\newcommand{\topRow}[1]{
        \subfigureWithTopCaption{#1}{left}{color}{-90}
        \subfigureWithTopCaption{#1}{left}{depth}{-90}\hfill
        \subfigureWithTopCaption{#1}{middle}{color}{180}
        \subfigureWithTopCaption{#1}{middle}{depth}{180}\hfill
        \subfigureWithTopCaption{#1}{right}{color}{-270}
        \subfigureWithTopCaption{#1}{right}{depth}{-270}\\
}

\newcommand{\middleRow}[1]{
        \subfigureWithoutCaption{#1}{left}{color}{-90}
        \subfigureWithoutCaption{#1}{left}{depth}{-90}\hfill
        \subfigureWithoutCaption{#1}{middle}{color}{180}
        \subfigureWithoutCaption{#1}{middle}{depth}{180}\hfill
        \subfigureWithoutCaption{#1}{right}{color}{-270}
        \subfigureWithoutCaption{#1}{right}{depth}{-270}\\
}

\newcommand{\bottomRow}[1]{
        \subfigureWithBottomCaption{#1}{left}{color}{-90}
        \subfigureWithBottomCaption{#1}{left}{depth}{-90}\hfill
        \subfigureWithBottomCaption{#1}{middle}{color}{180}
        \subfigureWithBottomCaption{#1}{middle}{depth}{180}\hfill
        \subfigureWithBottomCaption{#1}{right}{color}{-270}
        \subfigureWithBottomCaption{#1}{right}{depth}{-270}\\
}

\begin{figure*}
    \captionsetup[subfigure]{labelformat=empty}
    \topRow{apple}
    \foreach \object in {banana,binoculars,bowl,camera,cell_phone} {%
        \middleRow{\object}
    }
    \bottomRow{cup}
    \caption{Example RGB and depth images from ContactPose (`use' intention), with 3D joint locations projected into the images. Left hand joints are \textbf{\textcolor{OliveGreen}{green}}, right hand joints are \textbf{\textcolor{red}{red}} (continued below).}    
\end{figure*}

\begin{figure*}
    \ContinuedFloat
    \captionsetup[subfigure]{labelformat=empty}
    \topRow{door_knob}
    \foreach \object in {eyeglasses,flashlight,hammer,headphones,knife} {%
        \middleRow{\object}
    }
    \bottomRow{light_bulb}
    \caption{Example RGB and depth images from ContactPose (`use' intention), with 3D joint locations projected into the images. Left hand joints are \textbf{\textcolor{OliveGreen}{green}}, right hand joints are \textbf{\textcolor{red}{red}} (continued below).}    
\end{figure*}

\begin{figure*}
    \ContinuedFloat
    \captionsetup[subfigure]{labelformat=empty}
    \topRow{mouse}
    \foreach \object in {mug,pan,ps_controller,scissors,stapler} {%
        \middleRow{\object}
    }
    \bottomRow{toothbrush}
    \caption{Example RGB and depth images from ContactPose (`use' intention), with 3D joint locations projected into the images. Left hand joints are \textbf{\textcolor{OliveGreen}{green}}, right hand joints are \textbf{\textcolor{red}{red}} (continued below).}    
\end{figure*}

\begin{figure*}
    \ContinuedFloat
    \captionsetup[subfigure]{labelformat=empty}
    \topRow{toothpaste}
    \foreach \object in {utah_teapot,water_bottle} {%
        \middleRow{\object}
    }
    \bottomRow{wine_glass}
    \caption{Example RGB and depth images from ContactPose (`use' intention), with 3D joint locations projected into the images. Left hand joints are \textbf{\textcolor{OliveGreen}{green}}, right hand joints are \textbf{\textcolor{red}{red}}.}
    \label{fig:data_examples_rgbd}
\end{figure*}
}
{%
% object, position, mode, angle
\newcommand{\subfigureWithTopCaption}[3]{%
    \captionsetup[subfigure]{labelformat=empty}
    \begin{subfigure}{.23\textwidth}
        \caption{#2}
        \includegraphics[width=\linewidth]{supp_images/hand_contacts/#1_#2_hand#3.pdf}
    \end{subfigure}
}

% object, position, mode, angle
\newcommand{\subfigureWithoutCaption}[3]{%
    \captionsetup[subfigure]{labelformat=empty}
    \begin{subfigure}{.23\textwidth}
        \includegraphics[width=\linewidth]{supp_images/hand_contacts/#1_#2_hand#3.pdf}
    \end{subfigure}
}

% object, position, mode, angle
\newcommand{\subfigureWithBottomCaption}[3]{%
    \captionsetup[subfigure]{labelformat=empty}
    \begin{subfigure}{.23\textwidth}
        \includegraphics[width=\linewidth]{supp_images/hand_contacts/#1_#2_hand#3.pdf}
        \caption{#2}
    \end{subfigure}
}

\newcommand{\topRow}[1]{
    \subfigureWithTopCaption{#1}{use}{0}
    \subfigureWithTopCaption{#1}{use}{1}\hfill
    \subfigureWithTopCaption{#1}{handoff}{0}
    \subfigureWithTopCaption{#1}{handoff}{1}\hrule
}

\newcommand{\middleRow}[1]{
    \subfigureWithoutCaption{#1}{use}{0}
    \subfigureWithoutCaption{#1}{use}{1}\hfill
    \subfigureWithoutCaption{#1}{handoff}{0}
    \subfigureWithoutCaption{#1}{handoff}{1}\hrule
}

\newcommand{\bottomRow}[1]{
    \subfigureWithBottomCaption{#1}{use}{0}
    \subfigureWithBottomCaption{#1}{use}{1}\hfill
    \subfigureWithBottomCaption{#1}{handoff}{0}
    \subfigureWithBottomCaption{#1}{handoff}{1}\hrule
}

\begin{figure*}
    \captionsetup[subfigure]{labelformat=empty}
    \topRow{apple}
    \foreach \object in {banana,binoculars,bowl,camera} {%
        \middleRow{\object}
    }
    \bottomRow{cell_phone}
    \caption{Hand-part contact probabilities for objects in ContactPose (similarly to Figure 5 in the main paper, \textbf{\textcolor{red}{red}} indicates high probability and \textbf{\textcolor{blue}{blue}} indicates low probability) (continued below).}    
\end{figure*}

\begin{figure*}
    \ContinuedFloat
    \captionsetup[subfigure]{labelformat=empty}
    \topRow{cup}
    \foreach \object in {eyeglasses,flashlight,hammer,headphones} {%
        \middleRow{\object}
    }
    \bottomRow{knife}
    \caption{Hand-part contact probabilities for objects in ContactPose (similarly to Figure 5 in the main paper, \textbf{\textcolor{red}{red}} indicates high probability and \textbf{\textcolor{blue}{blue}} indicates low probability) (continued below).}    
\end{figure*}

\begin{figure*}
    \ContinuedFloat
    \captionsetup[subfigure]{labelformat=empty}
    \topRow{light_bulb}
    \foreach \object in {mouse,mug,pan,ps_controller} {%
        \middleRow{\object}
    }
    \bottomRow{scissors}
    \caption{Hand-part contact probabilities for objects in ContactPose (similarly to Figure 5 in the main paper, \textbf{\textcolor{red}{red}} indicates high probability and \textbf{\textcolor{blue}{blue}} indicates low probability) (continued below).}    
\end{figure*}

\begin{figure*}
    \ContinuedFloat
    \captionsetup[subfigure]{labelformat=empty}
    \topRow{stapler}
    \foreach \object in {toothbrush,toothpaste,utah_teapot,water_bottle} {%
        \middleRow{\object}
    }
    \bottomRow{wine_glass}
    \caption{Hand-part contact probabilities for objects in ContactPose (similarly to Figure 5 in the main paper, \textbf{\textcolor{red}{red}} indicates high probability and \textbf{\textcolor{blue}{blue}} indicates low probability). Data is grouped by left or right hand and by `use' or `hand-off' intent.}
    \label{fig:data_examples_hand_contacts}
\end{figure*}
}
{%
\begin{figure*}
    \centering
    \captionsetup[subfigure]{labelformat=empty}
    \foreach \num in {06,07,08,09,10,11,12,01,13,14,15,16,17,04,18,19,20,21,22,23,24,25,26,27} {%
        \vrule
        \foreach \view in {0,1} {%
            \begin{subfigure}{.155\textwidth}
                \includegraphics[width=\linewidth]{supp_images/grasps/object_slice/use/\num_\view.png}
            \end{subfigure}
        }\vrule
    }
    \caption{A slice through ContactPose: All PS-controller `use' grasps  (2 views per grasp) (continued below).}
\end{figure*}

\begin{figure*}
    \ContinuedFloat
    \centering
    \captionsetup[subfigure]{labelformat=empty}
    \foreach \num in {28,29,30,31,32,33,35,36,37,38,39,40,41,42,43,44,45,46,47,48,49,50} {%
        \vrule
        \foreach \view in {0,1} {%
            \begin{subfigure}{.155\textwidth}
                \includegraphics[width=\linewidth]{supp_images/grasps/object_slice/use/\num_\view.png}
            \end{subfigure}
        }\vrule
    }
    \caption{A slice through ContactPose: All PS-controller `use' grasps (2 views per grasp).}
    \label{fig:data_examples_grasps_use}
\end{figure*}

\begin{figure*}
    \centering
    \captionsetup[subfigure]{labelformat=empty}
    \foreach \num in {01,02,03,05,06,07,08,09,10,11,12,13,14,16,17,18,19,20,22,23,24,25,26,27} {%
        \vrule
        \foreach \view in {0,1} {%
            \begin{subfigure}{.155\textwidth}
                \includegraphics[width=\linewidth]{supp_images/grasps/object_slice/handoff/\num_\view.png}
            \end{subfigure}
        }\vrule
    }
    \caption{A slice through ContactPose: All PS-controller `hand-off' grasps  (2 views per grasp) (continued below).}
\end{figure*}

\begin{figure*}
    \ContinuedFloat
    \centering    
    \captionsetup[subfigure]{labelformat=empty}
    \foreach \num in {28,29,30,31,32,33,35,36,37,38,39,40,41,42,43,44,46,47,48,49,50} {%
        \vrule
        \foreach \view in {0,1} {%
            \begin{subfigure}{.155\textwidth}
                \includegraphics[width=\linewidth]{supp_images/grasps/object_slice/handoff/\num_\view.png}
            \end{subfigure}
        }\vrule
    }
    \caption{A slice through ContactPose: All PS-controller `hand-off' grasps  (2 views per grasp).}
    \label{fig:data_examples_grasps_handoff}
\end{figure*}
}
