# Supplementary material for: ContactPose: A Dataset of Grasps with Object Contact and Hand Pose
Source: arXiv:2007.09545 source file (2020-07-19)
Supplement: Supplementary file 2 [file data_examples_grasps_object_slice.tex]

{%
\begin{figure*}
    \centering
    \captionsetup[subfigure]{labelformat=empty}
    \foreach \num in {06,07,08,09,10,11,12,01,13,14,15,16,17,04,18,19,20,21,22,23,24,25,26,27} {%
        \vrule
        \foreach \view in {0,1} {%
            \begin{subfigure}{.155\textwidth}
                \includegraphics[width=\linewidth]{supp_images/grasps/object_slice/use/\num_\view.png}
            \end{subfigure}
        }\vrule
    }
    \caption{A slice through ContactPose: All PS-controller `use' grasps  (2 views per grasp) (continued below).}
\end{figure*}

\begin{figure*}
    \ContinuedFloat
    \centering
    \captionsetup[subfigure]{labelformat=empty}
    \foreach \num in {28,29,30,31,32,33,35,36,37,38,39,40,41,42,43,44,45,46,47,48,49,50} {%
        \vrule
        \foreach \view in {0,1} {%
            \begin{subfigure}{.155\textwidth}
                \includegraphics[width=\linewidth]{supp_images/grasps/object_slice/use/\num_\view.png}
            \end{subfigure}
        }\vrule
    }
    \caption{A slice through ContactPose: All PS-controller `use' grasps (2 views per grasp).}
    \label{fig:data_examples_grasps_use}
\end{figure*}

\begin{figure*}
    \centering
    \captionsetup[subfigure]{labelformat=empty}
    \foreach \num in {01,02,03,05,06,07,08,09,10,11,12,13,14,16,17,18,19,20,22,23,24,25,26,27} {%
        \vrule
        \foreach \view in {0,1} {%
            \begin{subfigure}{.155\textwidth}
                \includegraphics[width=\linewidth]{supp_images/grasps/object_slice/handoff/\num_\view.png}
            \end{subfigure}
        }\vrule
    }
    \caption{A slice through ContactPose: All PS-controller `hand-off' grasps  (2 views per grasp) (continued below).}
\end{figure*}

\begin{figure*}
    \ContinuedFloat
    \centering    
    \captionsetup[subfigure]{labelformat=empty}
    \foreach \num in {28,29,30,31,32,33,35,36,37,38,39,40,41,42,43,44,46,47,48,49,50} {%
        \vrule
        \foreach \view in {0,1} {%
            \begin{subfigure}{.155\textwidth}
                \includegraphics[width=\linewidth]{supp_images/grasps/object_slice/handoff/\num_\view.png}
            \end{subfigure}
        }\vrule
    }
    \caption{A slice through ContactPose: All PS-controller `hand-off' grasps  (2 views per grasp).}
    \label{fig:data_examples_grasps_handoff}
\end{figure*}
}
