# Supplementary material for: ContactPose: A Dataset of Grasps with Object Contact and Hand Pose
Source: arXiv:2007.09545 source file (2020-07-19)
Supplement: Supplementary file 3 [file data_examples_hand_contacts.tex]

{%
% object, position, mode, angle
\newcommand{\subfigureWithTopCaption}[3]{%
    \captionsetup[subfigure]{labelformat=empty}
    \begin{subfigure}{.23\textwidth}
        \caption{#2}
        \includegraphics[width=\linewidth]{supp_images/hand_contacts/#1_#2_hand#3.pdf}
    \end{subfigure}
}

% object, position, mode, angle
\newcommand{\subfigureWithoutCaption}[3]{%
    \captionsetup[subfigure]{labelformat=empty}
    \begin{subfigure}{.23\textwidth}
        \includegraphics[width=\linewidth]{supp_images/hand_contacts/#1_#2_hand#3.pdf}
    \end{subfigure}
}

% object, position, mode, angle
\newcommand{\subfigureWithBottomCaption}[3]{%
    \captionsetup[subfigure]{labelformat=empty}
    \begin{subfigure}{.23\textwidth}
        \includegraphics[width=\linewidth]{supp_images/hand_contacts/#1_#2_hand#3.pdf}
        \caption{#2}
    \end{subfigure}
}

\newcommand{\topRow}[1]{
    \subfigureWithTopCaption{#1}{use}{0}
    \subfigureWithTopCaption{#1}{use}{1}\hfill
    \subfigureWithTopCaption{#1}{handoff}{0}
    \subfigureWithTopCaption{#1}{handoff}{1}\hrule
}

\newcommand{\middleRow}[1]{
    \subfigureWithoutCaption{#1}{use}{0}
    \subfigureWithoutCaption{#1}{use}{1}\hfill
    \subfigureWithoutCaption{#1}{handoff}{0}
    \subfigureWithoutCaption{#1}{handoff}{1}\hrule
}

\newcommand{\bottomRow}[1]{
    \subfigureWithBottomCaption{#1}{use}{0}
    \subfigureWithBottomCaption{#1}{use}{1}\hfill
    \subfigureWithBottomCaption{#1}{handoff}{0}
    \subfigureWithBottomCaption{#1}{handoff}{1}\hrule
}

\begin{figure*}
    \captionsetup[subfigure]{labelformat=empty}
    \topRow{apple}
    \foreach \object in {banana,binoculars,bowl,camera} {%
        \middleRow{\object}
    }
    \bottomRow{cell_phone}
    \caption{Hand-part contact probabilities for objects in ContactPose (similarly to Figure 5 in the main paper, \textbf{\textcolor{red}{red}} indicates high probability and \textbf{\textcolor{blue}{blue}} indicates low probability) (continued below).}    
\end{figure*}

\begin{figure*}
    \ContinuedFloat
    \captionsetup[subfigure]{labelformat=empty}
    \topRow{cup}
    \foreach \object in {eyeglasses,flashlight,hammer,headphones} {%
        \middleRow{\object}
    }
    \bottomRow{knife}
    \caption{Hand-part contact probabilities for objects in ContactPose (similarly to Figure 5 in the main paper, \textbf{\textcolor{red}{red}} indicates high probability and \textbf{\textcolor{blue}{blue}} indicates low probability) (continued below).}    
\end{figure*}

\begin{figure*}
    \ContinuedFloat
    \captionsetup[subfigure]{labelformat=empty}
    \topRow{light_bulb}
    \foreach \object in {mouse,mug,pan,ps_controller} {%
        \middleRow{\object}
    }
    \bottomRow{scissors}
    \caption{Hand-part contact probabilities for objects in ContactPose (similarly to Figure 5 in the main paper, \textbf{\textcolor{red}{red}} indicates high probability and \textbf{\textcolor{blue}{blue}} indicates low probability) (continued below).}    
\end{figure*}

\begin{figure*}
    \ContinuedFloat
    \captionsetup[subfigure]{labelformat=empty}
    \topRow{stapler}
    \foreach \object in {toothbrush,toothpaste,utah_teapot,water_bottle} {%
        \middleRow{\object}
    }
    \bottomRow{wine_glass}
    \caption{Hand-part contact probabilities for objects in ContactPose (similarly to Figure 5 in the main paper, \textbf{\textcolor{red}{red}} indicates high probability and \textbf{\textcolor{blue}{blue}} indicates low probability). Data is grouped by left or right hand and by `use' or `hand-off' intent.}
    \label{fig:data_examples_hand_contacts}
\end{figure*}
}
