# Supplementary material for: ContactPose: A Dataset of Grasps with Object Contact and Hand Pose
Source: arXiv:2007.09545 source file (2020-07-19)
Supplement: Supplementary file 4 [file data_examples_rgbd.tex]

{%
\newcommand{\cameraName}[1]{
    \IfEqCase{#1}{%
        {left}{Kinect\#1}%
        {middle}{Kinect\#2}%
        {right}{Kinect\#3}%
    }[\PackageError{cameraName}{Undefined option to cameraName: #1}{}]%
}

% object, position, mode, angle
\newcommand{\subfigureWithTopCaption}[4]{%
    \captionsetup[subfigure]{labelformat=empty, font=tiny}
    \begin{subfigure}{.15\textwidth}
        \caption{\cameraName{#2}-#3}
        \includegraphics[width=\linewidth, angle=#4, origin=c]{supp_images/rgbd_images/#1_kinect2_#2_#3_use.png}
    \end{subfigure}
}

% object, position, mode, angle
\newcommand{\subfigureWithoutCaption}[4]{%
    \captionsetup[subfigure]{labelformat=empty}
    \begin{subfigure}{.15\textwidth}
        \includegraphics[width=\linewidth, angle=#4, origin=c]{supp_images/rgbd_images/#1_kinect2_#2_#3_use.png}
    \end{subfigure}
}

% object, position, mode, angle
\newcommand{\subfigureWithBottomCaption}[4]{%
    \captionsetup[subfigure]{labelformat=empty, font=tiny}
    \begin{subfigure}{.15\textwidth}
        \includegraphics[width=\linewidth, angle=#4, origin=c]{supp_images/rgbd_images/#1_kinect2_#2_#3_use.png}
        \caption{\cameraName{#2}-#3}
    \end{subfigure}
}

\newcommand{\topRow}[1]{
        \subfigureWithTopCaption{#1}{left}{color}{-90}
        \subfigureWithTopCaption{#1}{left}{depth}{-90}\hfill
        \subfigureWithTopCaption{#1}{middle}{color}{180}
        \subfigureWithTopCaption{#1}{middle}{depth}{180}\hfill
        \subfigureWithTopCaption{#1}{right}{color}{-270}
        \subfigureWithTopCaption{#1}{right}{depth}{-270}\\
}

\newcommand{\middleRow}[1]{
        \subfigureWithoutCaption{#1}{left}{color}{-90}
        \subfigureWithoutCaption{#1}{left}{depth}{-90}\hfill
        \subfigureWithoutCaption{#1}{middle}{color}{180}
        \subfigureWithoutCaption{#1}{middle}{depth}{180}\hfill
        \subfigureWithoutCaption{#1}{right}{color}{-270}
        \subfigureWithoutCaption{#1}{right}{depth}{-270}\\
}

\newcommand{\bottomRow}[1]{
        \subfigureWithBottomCaption{#1}{left}{color}{-90}
        \subfigureWithBottomCaption{#1}{left}{depth}{-90}\hfill
        \subfigureWithBottomCaption{#1}{middle}{color}{180}
        \subfigureWithBottomCaption{#1}{middle}{depth}{180}\hfill
        \subfigureWithBottomCaption{#1}{right}{color}{-270}
        \subfigureWithBottomCaption{#1}{right}{depth}{-270}\\
}

\begin{figure*}
    \captionsetup[subfigure]{labelformat=empty}
    \topRow{apple}
    \foreach \object in {banana,binoculars,bowl,camera,cell_phone} {%
        \middleRow{\object}
    }
    \bottomRow{cup}
    \caption{Example RGB and depth images from ContactPose (`use' intention), with 3D joint locations projected into the images. Left hand joints are \textbf{\textcolor{OliveGreen}{green}}, right hand joints are \textbf{\textcolor{red}{red}} (continued below).}    
\end{figure*}

\begin{figure*}
    \ContinuedFloat
    \captionsetup[subfigure]{labelformat=empty}
    \topRow{door_knob}
    \foreach \object in {eyeglasses,flashlight,hammer,headphones,knife} {%
        \middleRow{\object}
    }
    \bottomRow{light_bulb}
    \caption{Example RGB and depth images from ContactPose (`use' intention), with 3D joint locations projected into the images. Left hand joints are \textbf{\textcolor{OliveGreen}{green}}, right hand joints are \textbf{\textcolor{red}{red}} (continued below).}    
\end{figure*}

\begin{figure*}
    \ContinuedFloat
    \captionsetup[subfigure]{labelformat=empty}
    \topRow{mouse}
    \foreach \object in {mug,pan,ps_controller,scissors,stapler} {%
        \middleRow{\object}
    }
    \bottomRow{toothbrush}
    \caption{Example RGB and depth images from ContactPose (`use' intention), with 3D joint locations projected into the images. Left hand joints are \textbf{\textcolor{OliveGreen}{green}}, right hand joints are \textbf{\textcolor{red}{red}} (continued below).}    
\end{figure*}

\begin{figure*}
    \ContinuedFloat
    \captionsetup[subfigure]{labelformat=empty}
    \topRow{toothpaste}
    \foreach \object in {utah_teapot,water_bottle} {%
        \middleRow{\object}
    }
    \bottomRow{wine_glass}
    \caption{Example RGB and depth images from ContactPose (`use' intention), with 3D joint locations projected into the images. Left hand joints are \textbf{\textcolor{OliveGreen}{green}}, right hand joints are \textbf{\textcolor{red}{red}}.}
    \label{fig:data_examples_rgbd}
\end{figure*}
}
